# Supplementary material for: Extrinsic and intrinsic correlations in molecular information transmission
Source: arXiv:1602.08530 source file (2016-02-26)
Supplement: Supplementary file 1 [file SI_Mathematica.pdf]

# Extrinsic and intrinsic correlations in molecular information transmission

Vijay Singh[1,2] Martin Tchernookov[1,3] and Ilya Nemenman[1,4]
[1]Department of Physics, Emory University, Atlanta, GA 30322, USA
[2]Computational Neuroscience Initiative, University of Pennsylvania, Philadelphia, PA 19104, USA
[3]Department of Physics, Lamar University, Beaumont, TX 77710
[4]Department of Biology, Emory University, Atlanta, GA 30322, USA

# 1. DERIVATION OF EQUATION 3

### MUTUAL INFORMATION BETWEEN SIGNAL AND RESPONSE OF TWO INTERACTING UNITS

Assume that the signal $s$ and the responses of the two units $r_1$ and $r_2$ conditional on $s$ are all Gaussian, i.e.,

$$P(s) = \mathcal{N}\left(\bar{s}, {\sigma_s}^2\right)$$
$$P(r_1, r_2 \mid s) = \mathcal{N}\left((\bar{r}_1, \bar{r}_2), \Sigma\right),$$

here,
$\bar{s}$ and ${\sigma_s}^2$ are the mean and variance of the signal,
$(\bar{r}_1, \bar{r}_2)$ are the mean responses given the signal $s$,
$\Sigma = {\sigma_\eta}^2 \begin{pmatrix} 1 & \rho_\eta \\ \rho_\eta & 1 \end{pmatrix}$,
${\sigma_\eta}^2$ is the response variance conditional on the stimulus $s$, and
$\rho_\eta$ is the conditional correlation coefficient of the two responses.

Assuming that ${\sigma_s}^2$ is small, such that $\Sigma$ can be regarded as a constant, and
$r_i(s) = r_i(\bar{s}) + \partial_s r_i(\bar{s})\,(s - \bar{s})$,
the joint distribution is:

$$P(r_1, r_2) = \int ds\, P(r_1, r_2 \mid s) P(s) = \mathcal{N}\left((\bar{r}_1(\bar{s}), \bar{r}_2(\bar{s})), \tilde{\Sigma}\right)$$

where

$$\tilde{\Sigma} = \Sigma\left(1 + {\sigma_s}^2 \begin{bmatrix} \partial_s \bar{r}_1(s) \\ \partial_s \bar{r}_2(s) \end{bmatrix} \Sigma^{-1} \left[\partial_s \bar{r}_1(s),\ \partial_s \bar{r}_2(s)\right]\right)_{\bar{s}}$$

For a normal distribution, $\mathcal{N}(\mu, \Sigma)$, the entropy is $\frac{1}{2}\log|\Sigma|$ up to an additive constant, so we have the mutual information as

$$I[r_1, r_2; s] = S[r_1, r_2] - \langle S[r_1, r_2 \mid s] \rangle_{\bar{s}} = \frac{1}{2}\log\left[1 + \frac{(\partial_s \bar{r}(s))^2 \sigma^2{}_s}{(1 + \rho_\eta)\,\sigma^2{}_\eta}\right]_{\bar{s}}.$$

where we have chosen $\bar{r}_1 = \bar{r}_2 = \bar{r}$ for identical units.

For response linearly depending on $s$, this is equivalent to Eq. (4) in the main text.

# 2. Solution of the model using perturbation theory

### 1. The Generator Matrix and its Eigen-system

The tagged generator matrix is given as

```
TildeH[χ1_, χ2_, kin_, koff_, kabs_, khop_] := (−1) {{−2 kin, kabs Exp[ χ1] + koff, kabs Exp[ χ2] + koff, 0},
        {kin, −kin − kabs − koff − khop, khop, kabs Exp[ χ2] + koff},
        {kin, khop, −kin − kabs  − koff − khop, koff + kabs Exp[ χ1]}, {0, kin, kin, −2 kabs − 2 koff}};
MatrixForm[TildeH[χ1, χ2, kin, koff, kabs, khop]]
```

$$\begin{pmatrix} 2\,\text{kin} & -e^{\chi 1}\,\text{kabs}-\text{koff} & -e^{\chi 2}\,\text{kabs}-\text{koff} & 0 \\ -\text{kin} & \text{kabs}+\text{khop}+\text{kin}+\text{koff} & -\text{khop} & -e^{\chi 2}\,\text{kabs}-\text{koff} \\ -\text{kin} & -\text{khop} & \text{kabs}+\text{khop}+\text{kin}+\text{koff} & -e^{\chi 1}\,\text{kabs}-\text{koff} \\ 0 & -\text{kin} & -\text{kin} & 2\,\text{kabs}+2\,\text{koff} \end{pmatrix}$$

The original generator matrix is:

```
H  = TildeH[0, 0, kin, koff, kabs, khop]; MatrixForm[H]
```

$$\begin{pmatrix} 2\,\text{kin} & -\text{kabs}-\text{koff} & -\text{kabs}-\text{koff} & 0 \\ -\text{kin} & \text{kabs}+\text{khop}+\text{kin}+\text{koff} & -\text{khop} & -\text{kabs}-\text{koff} \\ -\text{kin} & -\text{khop} & \text{kabs}+\text{khop}+\text{kin}+\text{koff} & -\text{kabs}-\text{koff} \\ 0 & -\text{kin} & -\text{kin} & 2\,\text{kabs}+2\,\text{koff} \end{pmatrix}$$

The left and right Eigen-systems of the generator matrix is

```
ER = Eigensystem[H]
EL = Eigensystem[Transpose[H]]
```

$$\Big\{\{0,\ \text{kabs}+\text{kin}+\text{koff},\ 2\,(\text{kabs}+\text{kin}+\text{koff}),\ \text{kabs}+2\,\text{khop}+\text{kin}+\text{koff}\},$$
$$\Big\{\Big\{-\frac{-\text{kabs}^2-2\,\text{kabs}\,\text{koff}-\text{koff}^2}{\text{kin}^2},\ -\frac{-\text{kabs}-\text{koff}}{\text{kin}},\ -\frac{-\text{kabs}-\text{koff}}{\text{kin}},\ 1\Big\},$$
$$\Big\{-\frac{\text{kabs}+\text{koff}}{\text{kin}},\ -\frac{-\text{kabs}+\text{kin}-\text{koff}}{2\,\text{kin}},\ -\frac{-\text{kabs}+\text{kin}-\text{koff}}{2\,\text{kin}},\ 1\Big\},\ \{1,-1,-1,1\},\ \{0,-1,1,0\}\Big\}\Big\}$$

$$\Big\{\{0,\ \text{kabs}+\text{kin}+\text{koff},\ 2\,(\text{kabs}+\text{kin}+\text{koff}),\ \text{kabs}+2\,\text{khop}+\text{kin}+\text{koff}\},$$
$$\Big\{\{1,1,1,1\},\ \Big\{-\frac{\text{kin}}{\text{kabs}+\text{koff}},\ -\frac{-\text{kabs}+\text{kin}-\text{koff}}{2\,(\text{kabs}+\text{koff})},\ -\frac{-\text{kabs}+\text{kin}-\text{koff}}{2\,(\text{kabs}+\text{koff})},\ 1\Big\},$$
$$\Big\{\frac{\text{kin}^2}{(\text{kabs}+\text{koff})^2},\ -\frac{\text{kin}}{\text{kabs}+\text{koff}},\ -\frac{\text{kin}}{\text{kabs}+\text{koff}},\ 1\Big\},\ \{0,-1,1,0\}\Big\}\Big\}$$

The perturbative part to the original generator matrix can be obtained by taking the difference between the tagged generator matirix and the original generator martrix. The difference defined as “delTildeH” is

```
delTildeH = TildeH[χ1, χ2, kin, koff, kabs, khop] − TildeH[0, 0, kin, koff, kabs, khop]; MatrixForm[delTildeH]
```

$$\begin{pmatrix} 0 & \text{kabs}-e^{\chi 1}\,\text{kabs} & \text{kabs}-e^{\chi 2}\,\text{kabs} & 0 \\ 0 & 0 & 0 & \text{kabs}-e^{\chi 2}\,\text{kabs} \\ 0 & 0 & 0 & \text{kabs}-e^{\chi 1}\,\text{kabs} \\ 0 & 0 & 0 & 0 \end{pmatrix}$$

## 2. Corrected Eigenvalues and Eigenvectors

Using the eigensystem of the generator matrix and delTildeH, we can get the correction to the eigenvalues and eigenvectors usign pertuebation theory. The corrected eigenvalues are:

$$\text{Do}\Big[\lambda_i = \text{Simplify}\Big[\text{Part[ER, 1, i]} + \frac{1}{\text{(Part[EL, 2, i].Part[ER, 2, i])}} \big(\text{(Part[EL, 2, i].delTildeH.Part[ER, 2, i])} + \text{Sum}\big[\big(\big(\text{Part[EL, 2, i].delTildeH.Part[ER, 2, j]}\big) * \big(\text{Part[EL, 2, j].delTildeH.Part[ER, 2, i]}\big)\big) / \big(\text{Part[EL, 2, j].Part[ER, 2, j]}\big) * \big(\text{If}\big[j == i, 0, 1 / \big(\text{Part[ER, 1, i]} - \text{Part[ER, 1, j]}\big)\big]\big), \{j, 1, 4\}\big]\big)\Big], \{i, 1, 4\}\Big]$$

Similarly the corrected left and right eigen-vectors are:

$$\text{Do}\Big[\Big\{R_i = \text{Simplify}\Big[\frac{1}{\text{Sqrt[Part[EL, 2, i].Part[ER, 2, i]]}} \big(\text{Part[ER, 2, i]} + \text{Sum}\big[\big(\text{Part[ER, 2, j]} * \big(\text{Part[EL, 2, j].delTildeH.Part[ER, 2, i]}\big)\big) / \big(\text{Part[EL, 2, j].Part[ER, 2, j]}\big) * \text{If}\big[j == i, 0, 1 / \big(\big(\text{Part[ER, 1, i]} - \text{Part[ER, 1, j]}\big)\big)\big], \{j, 1, 4\}\big]\big)\Big],$$

$$L_i = \text{Simplify}\Big[\frac{1}{\text{Sqrt[Part[EL, 2, i].Part[ER, 2, i]]}} \big(\text{Part[EL, 2, i]} + \text{Sum}\big[\big(\big(\text{Part[EL, 2, i].delTildeH.Part[ER, 2, j]}\big) * \text{Part[EL, 2, j]}\big) / \big(\text{Part[EL, 2, j].Part[ER, 2, j]}\big) * \text{If}\big[j == i, 0, 1 / \big(\big(\text{Part[ER, 1, i]} - \text{Part[ER, 1, j]}\big)\big)\big], \{j, 1, 4\}\big]\big)\Big]\Big\}, \{i, 1, 4\}\Big]$$

---

## 3. Steady state occupation of the receptors (Equilibrium conditions)

The probability of occupation is given by the vector $\{P_{00}, P_{01}, P_{10}, P_{11}\}$. In steady state the probabity of occupation can be determined by solving the equation

$$P(t)\,H = 0$$

The solution is:

```
P0 = Simplify[Part[{P00, P01, P10, P11} /. Solve[{2 kin P00 + (−kabs − koff) P01 + (−koff − kabs) P10 == 0,
        −kin P00 + (koff + khop + kin + kabs) P01 − khop P10 + (−koff − kabs) P11 == 0,
        −kin P01 − kin P10 + (2 koff + 2 kabs) P11 == 0,
        P00 + P01 + P10 + P11 == 1}, {P00, P01, P10, P11}], 1]]
```

$$\left\{\frac{(\text{kabs} + \text{koff})^2}{(\text{kabs} + \text{kin} + \text{koff})^2}, \frac{\text{kin}\,(\text{kabs} + \text{koff})}{(\text{kabs} + \text{kin} + \text{koff})^2}, \frac{\text{kin}\,(\text{kabs} + \text{koff})}{(\text{kabs} + \text{kin} + \text{koff})^2}, \frac{\text{kin}^2}{(\text{kabs} + \text{kin} + \text{koff})^2}\right\}$$

---

## 4. Probablity generating function for $(Q_1, Q_2)$

$$\text{GenFun} = \text{Simplify}[\{1, 1, 1, 1\}.(\text{Sum}[\text{Exp}[-\lambda_i * t]\, L_i.\text{P0}\, R_i, \{i, 1, 4\}])];$$

---

## 5. Mean and Variance of $(Q_1, Q_2)$

By taking the derivative of the cumulant generating function, Log[GenFun], one can get the mean and the variances.

Mean number of accumulated molecules. $< Q_1 | k_{in} >$ or $< Q_2 | k_{in} >$

$$\text{Qmean} = \text{Simplify}[\text{D}[\text{Log}[\text{GenFun}], \chi 1] /. \{\chi 1 \to 0, \chi 2 \to 0\}]$$

$$\frac{\text{kabs kin t}}{\text{kabs} + \text{kin} + \text{koff}}$$

Variance $< \delta Q^2{}_1 | k_{in} >$ or $< \delta Q^2{}_2 | k_{in} >$

$$\delta\text{Qsq11} = \text{FullSimplify}[\text{D}[\text{D}[\text{Log}[\text{GenFun}], \chi 1], \chi 1] /. \{\chi 1 \to 0, \chi 2 \to 0\}]$$

$$\Big(e^{-(\text{kabs}+2\,\text{khop}+\text{kin}+\text{koff})\,t}\ \text{kabs kin} \Big(e^{(\text{kabs}+2\,\text{khop}+\text{kin}+\text{koff})\,t}\ \text{kabs}^5\ t + e^{(\text{kabs}+2\,\text{khop}+\text{kin}+\text{koff})\,t}\ (\text{kin}+\text{koff})^3\ (2\,\text{khop}+\text{kin}+\text{koff})^2\ t + e^{(\text{kabs}+2\,\text{khop}+\text{kin}+\text{koff})\,t}\ \text{kabs}^4\ (4\,\text{khop}+3\,\text{kin}+5\,\text{koff})\ t - \text{kabs}\Big(\text{kin}\,(\text{kin}+\text{koff})^2 + e^{2\,\text{khop}\,t}\ \text{kin}\,(2\,\text{khop}+\text{kin}+\text{koff})^2 - e^{(\text{kabs}+2\,\text{khop}+\text{kin}+\text{koff})\,t}\ (\text{kin}+\text{koff})\ (2\,\text{khop}+\text{kin}+\text{koff})\ ((\text{kin}+\text{koff})\ (3\,\text{kin}+5\,\text{koff}) + \text{khop}\ (4\,\text{kin}+6\,\text{koff}))\ t\Big) - 2\,\text{kabs}^2\Big(\text{kin}\,(\text{kin}+\text{koff}) + e^{2\,\text{khop}\,t}\ \text{kin}\,(2\,\text{khop}+\text{kin}+\text{koff}) - e^{(\text{kabs}+2\,\text{khop}+\text{kin}+\text{koff})\,t}\Big(6\,\text{khop}\,(\text{kin}+\text{koff})\,(\text{kin}+2\,\text{koff}) + (\text{kin}+\text{koff})^2\,(2\,\text{kin}+5\,\text{koff}) + \text{khop}^2\,(4\,\text{kin}+6\,\text{koff})\Big)\,t\Big) + \text{kabs}^3\Big(-\big(1+e^{2\,\text{khop}\,t}\big)\,\text{kin} + 2\,e^{(\text{kabs}+2\,\text{khop}+\text{kin}+\text{koff})\,t}\Big(2\,\text{khop}^2 + (\text{kin}+\text{koff})\,(2\,\text{kin}+5\,\text{koff}) + \text{khop}\,(5\,\text{kin}+8\,\text{koff})\Big)\,t\Big)\Big)\Big)\Big/\Big((\text{kabs}+\text{kin}+\text{koff})^4\,(\text{kabs}+2\,\text{khop}+\text{kin}+\text{koff})^2\Big)$$

Covariance $< \delta Q_1\ \delta Q_2 | k_{in} >$.

$$\delta\text{Qsq12} = \text{FullSimplify}[\text{D}[\text{D}[\text{Log}[\text{GenFun}], \chi 1], \chi 2] /. \{\chi 1 \to 0, \chi 2 \to 0\}]$$

$$\Big(e^{-(\text{kabs}+2\,\text{khop}+\text{kin}+\text{koff})\,t}\ \text{kabs}^2\ \text{kin}^2 \Big((\text{kin}+\text{koff})^2 - e^{2\,\text{khop}\,t}\,(2\,\text{khop}+\text{kin}+\text{koff})^2 - 2\,e^{(\text{kabs}+2\,\text{khop}+\text{kin}+\text{koff})\,t}\ \text{khop}\,(\text{kin}+\text{koff})\,(2\,\text{khop}+\text{kin}+\text{koff})\,t - \text{kabs}^2\Big(-1 + e^{2\,\text{khop}\,t} + 2\,e^{(\text{kabs}+2\,\text{khop}+\text{kin}+\text{koff})\,t}\ \text{khop}\ t\Big) + 2\,\text{kabs}\Big(\text{kin}+\text{koff} - e^{2\,\text{khop}\,t}\,(2\,\text{khop}+\text{kin}+\text{koff}) - 2\,e^{(\text{kabs}+2\,\text{khop}+\text{kin}+\text{koff})\,t}\ \text{khop}\,(\text{khop}+\text{kin}+\text{koff})\,t\Big)\Big)\Big)\Big/\Big((\text{kabs}+\text{kin}+\text{koff})^4\,(\text{kabs}+2\,\text{khop}+\text{kin}+\text{koff})^2\Big)$$

Covariance matrix.

$$\text{Sig} = \{\{\delta\text{Qsq11}, \delta\text{Qsq12}\}, \{\delta\text{Qsq12}, \delta\text{Qsq11}\}\};$$

## 6. Transformation from $(Q_1, Q_2)$ to $(Q_+, Q_-)$

Let us first express $(Q_1, Q_2)$ in terms of $(Q_+, Q_-)$.

$$\text{Solve}[\{\delta Q_+ == \text{Q1} + \text{Q2} - 2\,\text{Qmean},\ Q_- == \text{Q1} - \text{Q2}\}, \{\text{Q1}, \text{Q2}\}]$$

$$\Big\{\Big\{\text{Q1} \to \frac{\text{kabs kin t}}{\text{kabs}+\text{kin}+\text{koff}} + \frac{Q_-}{2} + \frac{\delta Q_+}{2},\ \text{Q2} \to -((-2\,\text{kabs kin t} + \text{kabs}\,Q_- + \text{kin}\,Q_- + \text{koff}\,Q_- - \text{kabs}\,\delta Q_+ - \text{kin}\,\delta Q_+ - \text{koff}\,\delta Q_+)/(2\,(\text{kabs}+\text{kin}+\text{koff})))\Big\}\Big\}$$

Now the term inside the exponential of the gaussian can be written as

$$\text{exponent} = \{\text{Q1} - \text{Qmean}, \text{Q2} - \text{Qmean}\}.\text{Inverse}[\text{Sig}].\{\text{Q1} - \text{Qmean}, \text{Q2} - \text{Qmean}\} /. \Big\{\Big\{\text{Q1} \to \frac{\text{kabs kin t}}{\text{kabs}+\text{kin}+\text{koff}} + \frac{Q_-}{2} + \frac{\delta Q_+}{2},\ \text{Q2} \to -((-2\,\text{kabs kin t} + \text{kabs}\,Q_- + \text{kin}\,Q_- + \text{koff}\,Q_- - \text{kabs}\,\delta Q_+ - \text{kin}\,\delta Q_+ - \text{koff}\,\delta Q_+)/(2\,(\text{kabs}+\text{kin}+\text{koff})))\Big\}\Big\};$$

Next we express the term inside the exponential in terms of $Q_+$ and $Q_-$, and collect the terms corresponding to $Q^2{}_+$ and $Q^2{}_-$

exponentSimplified = Simplify[Normal[Series[exponent, {δQ₊, 0, 3}]]]

$$\left\{\frac{1}{2\,\text{kabs kin}}\, e^{(\text{kabs}+2\,\text{khop}+\text{kin}+\text{koff})\,t}\,(\text{kabs}+\text{kin}+\text{koff})^2 \left(\left((\text{kabs}+2\,\text{khop}+\text{kin}+\text{koff})^2\,Q_-^2\right)\Big/\left(e^{(\text{kabs}+2\,\text{khop}+\text{kin}+\text{koff})\,t}\,\text{kabs}^3\,t + e^{(\text{kabs}+2\,\text{khop}+\text{kin}+\text{koff})\,t}\,(\text{kin}+\text{koff})\,(2\,\text{khop}+\text{kin}+\text{koff})^2\,t + e^{(\text{kabs}+2\,\text{khop}+\text{kin}+\text{koff})\,t}\,\text{kabs}^2\,(4\,\text{khop}+\text{kin}+3\,\text{koff})\,t + \text{kabs}\left(e^{(\text{kabs}+2\,\text{khop}+\text{kin}+\text{koff})\,t}\,\text{kin}^2\,t + e^{(\text{kabs}+2\,\text{khop}+\text{kin}+\text{koff})\,t}\left(4\,\text{khop}^2+8\,\text{khop koff}+3\,\text{koff}^2\right)t + \text{kin}\left(-2+4\,e^{(\text{kabs}+2\,\text{khop}+\text{kin}+\text{koff})\,t}\,(\text{khop}+\text{koff})\,t\right)\right)\right) + \left((\text{kabs}+\text{kin}+\text{koff})^2\,\delta Q_+^2\right)\Big/\left(-2\,e^{2\,\text{khop}\,t}\,\text{kabs kin} + e^{(\text{kabs}+2\,\text{khop}+\text{kin}+\text{koff})\,t}\left(\text{kabs}^3+(\text{kin}+\text{koff})^3+\text{kabs}^2\,(\text{kin}+3\,\text{koff})+\text{kabs}\left(\text{kin}^2+4\,\text{kin koff}+3\,\text{koff}^2\right)\right)t\right)\right)\right\}$$

$< \delta Q^2{}_+ \mid k_{in} >$ can be obtained as the inverse of the coefficient of the term corresponding to $\delta Q^2{}_+$.

varδQsum = 1 / Coefficient[exponentSimplified, δQ₊²]

$$\left\{\frac{1}{(\text{kabs}+\text{kin}+\text{koff})^4}\,2\,e^{-(\text{kabs}+2\,\text{khop}+\text{kin}+\text{koff})\,t}\,\text{kabs kin}\left(-2\,e^{2\,\text{khop}\,t}\,\text{kabs kin} + e^{(\text{kabs}+2\,\text{khop}+\text{kin}+\text{koff})\,t}\left(\text{kabs}^3+(\text{kin}+\text{koff})^3+\text{kabs}^2\,(\text{kin}+3\,\text{koff})+\text{kabs}\left(\text{kin}^2+4\,\text{kin koff}+3\,\text{koff}^2\right)\right)t\right)\right\}$$

$< \delta Q^2{}_- \mid k_{in} >$ can be obtained as the inverse of the coefficient of the term corresponding to $Q^2{}_-$.

varδQdiff = 1 / Coefficient[exponentSimplified, Q₋²]

$$\left\{\left(2\,e^{-(\text{kabs}+2\,\text{khop}+\text{kin}+\text{koff})\,t}\,\text{kabs kin}\left(e^{(\text{kabs}+2\,\text{khop}+\text{kin}+\text{koff})\,t}\,\text{kabs}^3\,t + e^{(\text{kabs}+2\,\text{khop}+\text{kin}+\text{koff})\,t}\,(\text{kin}+\text{koff})\,(2\,\text{khop}+\text{kin}+\text{koff})^2\,t + e^{(\text{kabs}+2\,\text{khop}+\text{kin}+\text{koff})\,t}\,\text{kabs}^2\,(4\,\text{khop}+\text{kin}+3\,\text{koff})\,t + \text{kabs}\left(e^{(\text{kabs}+2\,\text{khop}+\text{kin}+\text{koff})\,t}\,\text{kin}^2\,t + e^{(\text{kabs}+2\,\text{khop}+\text{kin}+\text{koff})\,t}\left(4\,\text{khop}^2+8\,\text{khop koff}+3\,\text{koff}^2\right)t + \text{kin}\left(-2+4\,e^{(\text{kabs}+2\,\text{khop}+\text{kin}+\text{koff})\,t}\,(\text{khop}+\text{koff})\,t\right)\right)\right)\right)\Big/\left((\text{kabs}+\text{kin}+\text{koff})^2\,(\text{kabs}+2\,\text{khop}+\text{kin}+\text{koff})^2\right)\right\}$$

In the long time limit, t -> ∞, these can be written as

Assuming[kin > 0 && kabs > 0 && khop > 0 && koff > 0, Limit[varδQsum/t, t → ∞]]

$$\left\{\left(2\,\text{kabs kin}\left(\text{kabs}^2+2\,\text{kabs koff}+(\text{kin}+\text{koff})^2\right)\right)\Big/(\text{kabs}+\text{kin}+\text{koff})^3\right\}$$

Assuming[kin > 0 && kabs > 0 && khop > 0 && koff > 0, Limit[varδQdiff/t, t → ∞]]

$$\left\{\left(2\,\text{kabs kin}\left(\text{kabs}^2+2\,\text{kabs}\,(\text{khop}+\text{koff})+(\text{kin}+\text{koff})\,(2\,\text{khop}+\text{kin}+\text{koff})\right)\right)\Big/\left((\text{kabs}+\text{kin}+\text{koff})^2\,(\text{kabs}+2\,\text{khop}+\text{kin}+\text{koff})\right)\right\}$$

The last two expressions are the variance of $J_+$ and $J_-$ as given in the main text.
